# Supplementary material for: CobWeb: A Research Prototype for Exploring User Bias in Political Fact-Checking
Source: arXiv:1907.03718 source file (2019-07-08)
Supplement: Supplementary file 1 [file appendix.tex]

\appendix

\section{Headings in Appendices}
The rules about hierarchical headings discussed above for
the body of the article are different in the appendices.
In the \textbf{appendix} environment, the command
\textbf{section} is used to
indicate the start of each Appendix, with alphabetic order
designation (i.e., the first is A, the second B, etc.) and
a title (if you include one).  So, if you need
hierarchical structure
\textit{within} an Appendix, start with \textbf{subsection} as the
highest level. Here is an outline of the body of this
document in Appendix-appropriate form:
\subsection{Introduction}
\subsection{The Body of the Paper}
\subsubsection{Type Changes and  Special Characters}
\subsubsection{Math Equations}
\paragraph{Inline (In-text) Equations}
\paragraph{Display Equations}
\subsubsection{Citations}
\subsubsection{Tables}
\subsubsection{Figures}
\subsubsection{Theorem-like Constructs}
\subsubsection*{A Caveat for the \TeX\ Expert}

% This next section command marks the start of
% Appendix B, and does not continue the present hierarchy
\section{Additional Documentation}
The file \path{acmart.pdf} contains both the user guide and the commented code.

\section{Matt's Helpful Appendix}

This appendix just shows examples of how to use \LaTeX.  We will cut it  and not ship it.

Each paragraph should have a blank line between them in the source.  Note the first paragraph of each section is automatically unindented, while subsequent paragraphs are indented. 

``Short quotations are marked by 2 back-tilde's at the start and 2 apostrophes at the end''

\begin{quotation}
Long quotations can be indented without quotation marks.
\end{quotation}

Websites are typically footnoted\footnote{\url{http://cikm2016.cs.iupui.edu}}.

Examples of comments shown in source code and not visible here when rendered.
% comment
\begin{comment}
more
comments 
here
\end{comment}

{\bf Editing notes}. %Use todo notes to help point out where more work is needed without breaking the flow of the main text. 
You can also \hl{highlight text}. In addition, there are a few editing commands to mark \st{strike-through text}, note text \add{to add}, or text to \replace{keep}{replace}. \todo{A thing to do} \ml{Something for ML todo} \ab{something for AB to do}

{\bf Avoid contractions}. In academic writing, avoid contractions (e.g., can't, didn't, he'll, I'll, needn't, we'll, won't, wouldn't, etc.) and write out full words (e.g., cannot, did not, he will, I will, need not, we will, will not, would not, etc.).

{\bf Cross-references}. Do not type cross-references to other sections explicitly; use cross-references which will automatically fill-in appropriate section numbers as sections move and change.  For example,  Section \ref{section:subsection-example}, Section \ref{section:subsubsection-example}, Figure \ref{myfigure}, Tables \ref{table:foo} and \ref{table:example}, and Equation \ref{equation:example}.

%---------------------------------------
\subsection{Subsection Example}
\label{section:subsection-example}

Sections can have subsections.  This is an example.

%---------------------------------------
\subsubsection{SubSubsection Example}
\label{section:subsubsection-example}

subsubsection text.

\paragraph{Paragraph headings} Paragraph headings can be used to emphasize a conceptual theme of a paragraph or for subsubsections.

This is a numbered equation:
\begin{align} 
\label{equation:example}
a^2+b^2=c^2
\end{align}

This is an unnumbered equation:
\begin{align*}
a^2+b^2=c^2
\end{align*}

You can also embed math in a sentence, e.g., $a+b=c$.

%---------------------------------------
\subsection{How to Add citations}
\label{section:citation-examples}

\begin{table} 
\begin{center}
\caption{ This is an example of table.}
\begin{tabular}{|l|l|l|c|c|}
\hline
\bf Collection & \bf \# Docs & \bf Topics \\
\hline
Robust04 & 528,155 & 301-450,601-700 \\
W10g & 1,692,096 & 451-550 \\
GOV2 & 25,205,179 & 701-850 \\
\hline
\end{tabular}
\label{table:foo}
\end{center}
\end{table} 

Do not explicitly type citations. Instead, use citation commands which will not only format citations correctly, but update if text in bibliography entry changes, and automatically populate bibliography with entries for all cited works. 

\noindent We can also extract the author names or year of a citation to include in the text of a sentence, e.g.,
\begin{itemize}
\item {\tt citeauthor} inserts author name(s) only: \citeauthor{smith2013dirt} were early pioneers.
\item {\tt citeyear} inserts publication year only: Work began as early as \citeyear{smith2013dirt}.
\item {\tt cite} inserts the reference number only: great work was done \cite{smith2013dirt}. Do NOT use the reference number as the noun in a sentence, e.g., ``\cite{smith2013dirt} did good work.''
\item {\tt citet} inserts the author name(s) and reference number: \citet{smith2013dirt} did great work!
\end{itemize}

%----------------------------------------------------------
% For tables use
\begin{table}
\begin{center}
% table caption is above the table
\caption{Please write your table caption here}
\label{table:example}       
% For LaTeX tables use
\begin{tabular}{lll}
\hline\noalign{\smallskip}
first & second & third  \\
\noalign{\smallskip}\hline\noalign{\smallskip}
number & number & number \\
number & number & number \\
\noalign{\smallskip}\hline
\end{tabular}
\end{center}
\end{table}

This is an example of an embedded figure. It should be formatted as "figure". Also it should have a caption with title and description. The caption should be centered under the figure with no empty line in between.
\begin{figure}[ht]
\centerline{\includegraphics[width=0.45\textwidth]{figures/NonArabic.png}} % Give the name of the image here.
\caption{Figure caption goes here.} %Please note that you will need to manually write out the full reference of the work here as it would be shown in the Reference section, plus the copyright note too if you are referencing something.Use the example for reference.
\label{myfigure}
\end{figure}
